# Supplementary material for: I2V3D: Controllable image-to-video generation with 3D guidance
Source: arXiv:2503.09733 source file (2025-03-12)
Supplement: Supplementary file 1 [file X_suppl.tex]

\clearpage

\setcounter{page}{1}
\maketitlesupplementary
\appendix

\section{User Study}~\label{user_study}
In this section, we further conduct a user study to evaluate the effectiveness of our approach. We compare our method with the baselines mentioned for both human-like characters videos (AnimateAnyone~\cite{hu2024animate}, MagicPose~\cite{chang2023magicpose}, ISculpting~\cite{yenphraphai2024image}) and nonhuman-like object videos (DragAnything~\cite{wu2025draganything}, MotionBooth~\cite{wu2024motionbooth}, ISculpting~\cite{yenphraphai2024image}).

The user study includes 30 animations. For each animation, participants were shown the original input image and rendered videos, followed by animations generated by the baseline methods and our approach, arranged in random order. Each animation was repeated three times to ensure participants had ample time to assess and compare the results. Participants were then asked to answer three questions by selecting the best option:

\begin{itemize}
    \item \textbf{Alignment:} Select the video that best preserves the motion of the objects and camera in the rendered video and the appearance of the input image.
    \item \textbf{Consistency:} Select the video with the least flicker.
    \item \textbf{Overall quality:} Select the video with the fewest artifacts.
\end{itemize}

We collected a total of 24 questionnaires from participants aged 20 to 55, including 7 with CG and CV backgrounds and 17 from other fields. The results of the user study, as shown in Fig.~\ref{fig:userstudy}, indicate that our method outperforms the other methods in all three factors. It achieved preferred rates of 0.811 and 0.814 for alignment, 0.856 and 0.814 for consistency, and 0.844 and 0.828 for video quality.

\section{Ablation Study}~\label{supp_abl}

% \noindent\textbf{Single Stage vs. Two Stages. } Fig.~\ref{fig:ablation_single} shows that the single-stage approach struggles when the first and subsequent frames differ significantly, causing texture loss (e.g., the sea turtle) and color shifts (e.g., the water), while our two-stage method preserves visual details.
\noindent\textbf{Single Stage vs. Two Stages. }  We conducted an ablation study using a single-stage approach, where the input image served as the first frame, and geometric guidance was applied as described in Sec.\ref{interpolation}. As shown in third row of Fig.\ref{fig:ablation_single}, the sea turtle loses texture because the image-to-video model struggles when the first and subsequent frames differ substantially. Moreover, the water color shifts over time due to accumulated errors, whereas our two-stage approach preserves the input image's visual details throughout the entire video sequence.

\noindent\textbf{Reconstructed 3D Background Meshes.} As discussed in Sec.\ref{sec: reconstruct}, we reconstruct the mesh for the background as well, which offers two key advantages. First, reconstructed meshes enable meaningful interactions with the background. For instance, as shown in the first panel of Fig.\ref{fig:abl_mesh}, our method allows the goose to walk behind the fire hydrant, even when it is partially occluded. In contrast, using the image plane as the background restricts the goose to the frontal plane, causing it to block the fire hydrant rather than moving behind it. Second, the reconstructed background meshes provide 3D guidance after camera movement. By comparison, relying on the image plane results in an invisible black region when the camera moves, as shown in the second panel of Fig.~\ref{fig:abl_mesh}, where the camera moves backward. While the diffusion model can fill in the black region using its generalization capability, the generated content is often unrealistic, such as additional goal frames or soccer balls. In contrast, our reconstructed meshes guide the expanded scene, ensuring that the result is more realistic. Third, background reconstruction facilitates large camera movement in video generation, as shown in Fig.~\ref{fig:camera_move}.

\noindent\textbf{3D-Guided Video Generation vs. Video Refinement}  We also conduct an ablation study using video refinement to evaluate the effectiveness of our 3D-guided video generation method, as shown in Fig.~\ref{fig:abl_v2v}. Following the Renoise strategy~\cite{meng2021sdedit, feng2025explorative}, we add random noise to the video up to a certain noise level and then denoise it to obtain refined images. Specifically, we use SVD~\cite{blattmann2023stable}, adopting the input image as the first frame and setting $t$ to 0.4. However, this approach fails to correct the background region, and due to the discontinuity between the first frame and subsequent frames, it results in noticeable blurriness. Additionally, we apply TokenFlow~\cite{geyer2023tokenflow}, a video-to-video translation method based on a text-to-image diffusion model. For a fair comparison, we use our fine-tuned SDXL LoRA. The results indicate that despite these refinements, noticeable flickering issues persist. In contrast, our method outperforms these approaches by effectively reducing artifacts while maintaining the smoothness of the video. 

%By using this method, users can set multiple camera keyframes in the 3D scene to create a complex moving trajectory as shown in Fig.~\ref{fig:camera_move}.

\section{Limitations}

Despite the effectiveness of our method, it has three main limitations. First, it cannot fully resolve artifacts caused by inaccurate 3D reconstruction, especially when geometric errors are significant. For example, the human hands in Fig.\ref{fig:limitation}, first row, exhibit distortions that stem from inaccurately reconstructed geometry. Second, the detailed appearance of objects in the generated video does not always perfectly align with the input image. The discrepancy, such as the variation from paper to leaf in Fig. \ref{fig:limitation}, second row, arises from the limited capability of customizing a diffusion model with LoRA to capture fine-grained details. Lastly, the generated video is not entirely smooth, as some small flickering persists. This reflects the limitations of current open-source video diffusion models. Fortunately, since our I2V3D framework is general and not tied to specific reconstruction and generation models, we believe these problems can be addressed with advancements in 3D modeling techniques and improved image \cite{flux, esser2024scaling} and video generation models \cite{yang2024cogvideox}.

% \begin{minipage}[t]{0.48\textwidth}
%     \centering
%     \includegraphics[width=\linewidth]{Figures/abl_single.jpg}
%     \captionsetup{skip=1pt} % 调整caption和图片的间距
%     \caption{Ablation on single-stage and two-stage video generation. The red boxes highlight texture loss and error accumulation.}
%     \label{fig:ablation_single}
%   \end{minipage}

\begin{figure}[tbp]
  \centering
  \begin{minipage}[t]{0.48\textwidth}
    \centering
    \includegraphics[width=\linewidth]{Figures/abl_single.jpg}
    \captionsetup{skip=1pt} % 调整caption和图片的间距
    \caption{Ablation on single-stage and two-stage video generation. The red boxes highlight texture loss and error accumulation.}
    \label{fig:ablation_single}
  \end{minipage}

  \vspace{0.5em} % 调整垂直间距
  \begin{minipage}[t]{0.48\textwidth}
    \centering
    \includegraphics[width=\linewidth]{Figures/abl_mesh.jpg}
    \captionsetup{skip=1pt} % 调整caption和图片的间距
      \caption{Ablation on 3D reconstruction for background. Scene A and B are w/o and w/ background reconstruction respectively.}
      \label{fig:abl_mesh}
  \end{minipage}
  
  \vspace{0.5em} % 调整垂直间距

   \begin{minipage}[t]{0.48\textwidth}
    \centering
    \includegraphics[width=\linewidth]{Figures/user_study.jpg}
    \captionsetup{skip=1pt} % 调整caption和图片的间距
      \caption{Results of user study. Our method has the best preferred rate for all video alignment, consistency and quality on both human-like characters and nonhuman-like objects..}
      \label{fig:userstudy}
  \end{minipage}
\end{figure}

\begin{figure}[htp]
  \centering
  \captionsetup{skip=3pt}
  \includegraphics[width=1.0\linewidth]{Figures/abl_v2v.jpg}
  \caption{Ablation on 3D-guided video generation vs. video refinement. The red boxes highlight failures in refinement.}
  \label{fig:abl_v2v}
\end{figure}

\begin{figure}[htp]
  \centering
  \captionsetup{skip=3pt}
  \includegraphics[width=1.0\linewidth]{Figures/more_results.jpg}
  \caption{Generate video with large camera movement.}
  \label{fig:camera_move}
\end{figure}

\begin{figure}[htp]
  \centering
  \captionsetup{skip=3pt}
  \includegraphics[width=1.0\linewidth]{Figures/limitation.jpg}
  \caption{Our limitations. 1st row: Artifacts caused by the coarseness of the reconstructed mesh. 2nd row: insufficient customization provided by LoRA.}
    \label{fig:limitation}
\end{figure}

% \begin{figure}[hbp]
%   \centering
%   \captionsetup{skip=3pt}
%   \includegraphics[width=1.0\linewidth]{Figures/user_study.jpg}
%   \caption{Results of user study. Our method has the best preferred rate for all video alignment, consistency and quality on both human-like characters and nonhuman-like objects.}
%   \label{fig:userstudy}
% \end{figure}
